# Supplementary material for: Piecewise Interaction Picture Density Matrix Quantum Monte Carlo
Source: arXiv:2108.06252 source file (2022-04-08)
Supplement: Supplementary file 1 [file si.pdf]

# Supporting Information for: "Piecewise Interaction Picture Density Matrix Quantum Monte Carlo"

William Van Benschoten[1] and James J. Shepherd[1, a)]
*Department of Chemistry, University of Iowa*

(Dated: April 8, 2022)

## I. PROPAGATION

Our description of propagation below follows the text due to Malone.[1]

In DMQMC the propagation equation is the symmetrized Bloch equation,

$$\frac{\mathrm{d}\hat{f}(\tau)}{\mathrm{d}\tau} = -\frac{1}{2}\left[\hat{H}\hat{f}(\tau) + \hat{f}(\tau)\hat{H}\right], \tag{1}$$

and propagating with a finite $\Delta\tau$ yields the equations of motion:

$$f_{ij}(\tau + \Delta\tau) = f_{ij}(\tau)\left[1 + \Delta\tau S\right] - \frac{\Delta\tau}{2}\sum_k \left[H_{ik} f_{kj}(\tau) + f_{ik}(\tau) H_{kj}\right], \tag{2}$$

where $S$ is a constant shift applied to each matrix element to control the walker population.

In general, stochastic spawning/removal of walkers is defined as follows. A random number, $r$, is drawn from a uniform distribution from 0 to 1. Then, if the 'probability' $p$ is greater than $r$, a walker is added or subtracted depending on the sign convention. If $p > 1$ then the integer component of $p$ is spawned directly and then the remainder after this is subject to the random number test above.

The propagator is interpreted in the following way:

1. Spawning: For a walker on $f_{ij}$ with a sign defined by sign($f_{ij}$), an element $f_{kj}$ is selected with a random uniform probability over available connected $k$ ($i \neq k$). The probability of such a connection, $p_{\text{gen}}$, is defined by the inverse of the number of possible one- and two-particle excitations. The probability of spawning is set to $\frac{\Delta\tau}{2p_{gen}} \mid H_{ik} \mid$ and the sign comes from: $\text{sign}(f_{kj}) = \text{sign}(f_{ij}) \times \text{sign}(H_{ik})$ The same process is repeated to spawn from $f_{ij}$ to $f_{ik}$.

2. Death/Cloning: For a walker on $f_{ij}$, the death/cloning probability is given as: $p_d = \Delta\tau(S - \frac{1}{2}\left[H_{ii} + H_{jj}\right])$. The removed/added walkers have the sign: $\text{sign}(S - \frac{1}{2}\left[H_{ii} + H_{jj}\right]) \times \text{sign}(f_{ij})$.

3. Annihilation: Walkers on $f_{ij}$ with opposite signs annihilate, leaving walkers of a single sign on $f_{ij}$.

a) Electronic mail: james-shepherd@uiowa.edu

In IP-DMQMC the equation of motion is,

$$f_{ij}(\tau + \Delta\tau) = f_{ij}(\tau)\left[1 + \Delta\tau S\right] - \Delta\tau \sum_k \left[-H^{(0)}_{ik} f_{kj}(\tau) + f_{ik}(\tau) H_{kj}\right]. \tag{3}$$

where the shift ($S$) serves the same function as in DMQMC. This is interpreted through the following steps performed while looping over each walker:

1. Spawning: Proceeds as with DMQMC, but only has probability $\frac{\Delta\tau}{p_{gen}} \mid H_{kj} \mid$ and does not spawn twice.

2. Death/Cloning: Proceeds as with DMQMC but the $p_d = \Delta\tau\left[S + H^{(0)}_{ii} - H_{jj}\right]$ is used instead.

3. Annihilation: Proceeds as with DMQMC.

The shift ($S$) is updated every $A$ times the steps described above have been applied, and is controlled through the simulations input file. In this work we used $A = 10$. The equation used in this work to update the shift is provided in the manuscript and was as described in the original DMQMC paper.[2]

## II. CALCULATION DETAILS

All simulations use a $\Delta\tau = 0.001$, the shift is updated and data is reported every 10 iterations.

The $N_\beta$ and $N_w$ pairings are found in Table II for the initiator PIP-DMQMC simulations. With the exception of $H_2O$/cc-pVDZ for $N_w = 5 \times 10^8$ and HBCH2$_2$/STO-3G for $N_w = 5 \times 10^7$, only 4 $\beta$-loops were collected due to computational cost considerations. The $HBCH_2$/STO-3G system was run with walker populations $N_w = 5 \times 10^4$, $5 \times 10^5$, $5 \times 10^6$ and $N_w = 5 \times 10^7$. Both $CH_4$/cc-pVDZ and $H_2O$/cc-pVDZ were run with walker populations $N_w = 5 \times 10^6 \to 5 \times 10^8$.

All integral dump files are generated using Molpro.[12] Single particle eigenvalues are include in integral files and are generated with the relevant equations.[13]

Geometries are presented in Table I. For $HBCH_2$ additional precision is present in the geometries which come from a Gaussian09 calculation.[9]

The walker population typically does not remain exactly at the population used in the simulation input file. The average minimum and average maximum of each simulation is reported in Table II.

## III. SUPPLEMENTARY FIGURES

Figures Fig. 1 and Fig. 2 show full scheme PIP-DMQMC simulations. Figure 3 shows ground-state initiator FCIQMC convergence plots for $H_2O$/cc-pVDZ and $CH_4$/cc-pVDZ.

## REFERENCES


[1] F. D. Malone, *Quantum Monte Carlo Simulations of Warm Dense Matter*, Ph.D. thesis (2017).
[2] N. S. Blunt, T. W. Rogers, J. S. Spencer, and W. M. C. Foulkes, Physical Review B **89**, 245124 (2014).
[3] P. F. Bernath, A. Shayesteh, K. Tereszchuk, and R. Colin, Science **297**, 1323 (2002).
[4] H. R. Petras, W. Z. Van Benschoten, S. K. Ramadugu, and J. J. Shepherd, Journal of Chemical Theory and Computation **17**, 6036 (2021).
[5] G. Herzberg, *Electronic spectra and electronic structure of polyatomic molecules*, Vol. 3 (van Nostrand, 1966).
[6] L. Wharton, W. Klemperer, L. P. Gold, R. Strauch, J. J. Gallagher, and V. E. Derr, The Journal of Chemical Physics **38**, 1203 (1963).
[7] F. Lovas, "Diatomic Spectral Database, NIST Standard Reference Database 114," (2002), type: dataset.
[8] G. H. Booth, A. J. W. Thom, and A. Alavi, The Journal of Chemical Physics **131**, 054106 (2009).
[9] M. Frisch, G. Trucks, H. B. Schlegel, G. E. Scuseria, M. A. Robb, J. R. Cheeseman, G. Scalmani, V. Barone, B. Mennucci, G. Petersson, and others, Inc., Wallingford CT **201** (2009).
[10] R. D. Johnson and others, http://srdata.nist.gov/cccbdb (2006).
[11] H. R. Petras, S. K. Ramadugu, F. D. Malone, and J. J. Shepherd, Journal of Chemical Theory and Computation **16**, 1029 (2020).
[12] H.-J. Werner, P. J. Knowles, G. Knizia, F. R. Manby, M. Schütz, and others, "MOLPRO, 2019.2 , a package of ab initio programs," (2019), see https://www.molpro.net.
[13] A. Szabo and N. S. Ostlund, *Modern quantum chemistry: introduction to advanced electronic structure theory* (Courier Corporation, 2012).

Table I. Distances and angles between the atoms of the molecules used in the manuscript and in Figures 1-3.

| Molecule | Basis set | Distances and Angles | Ref. |
|---|---|---|---|
| $BeH_2$ | Be/cc-pVDZ<br>H/DZ | Be–H: 1.33376Å<br>∠HBeH: 180° | 3 |
| equilibrium $H_4$ | cc-pVDZ | H–H: 0.945110567Å | 4 |
| equilibrium $H_8$ | STO-3G | H–H: 0.945110567Å | 4 |
| HCN | STO-3G | H–C: 1.064Å<br>C–N: 1.156Å<br>∠HCN: 180° | 5 |
| LiF | STO-3G | Li–F: 1.564Å | 6, 7 |
| $N_2$ | STO-3G | N–N: 2.068$a_0$ | 8 |
| stretched $H_8$ | STO-3G | H–H: 1.270025398Å | 4 |
| $HBCH_2$ | STO-3G | C–B: 1.33825301Å<br>C–H: 1.0788872Å<br>B–H: 1.14721397Å<br>∠HCB: 122.82860383°<br>∠CBH: 179.99999852° | 9, 10 |
| $H_2O$ | cc-pVDZ | O–H: 0.96Å<br>∠HOH: 109.5° | 11 |
| $CH_4$ | cc-pVDZ | C–H: 1.087728Å<br>∠HCH: 109.47122° | 8 |

Table II. A table of information summarizing the walker population dynamics for each calculation, organized by system and method in the first and second columns respectively. Unless parenthetically provided in the 'System' column, the PIP-DMQMC simulations use $\beta_T = 1.0$. To make comparisons easier we provide the intended initial walker population (input $N_w$), the true average initial walker population ($N_w(\beta = 0)$), the average of the minimum walker population from individual trajectories (Average min($N_w(\beta)$)), the average of the maximum walker population from individual trajectories (Average max($N_w(\beta)$)) and the total number of trajectories ($N_\beta$). Where applicable, the standard error is given in parenthesis next to the uncertain digit.

| System | Method | input $N_w$ | $N_w(\beta = 0)$ | Average min($N_w(\beta)$) | Average max($N_w(\beta)$) | $N_\beta$ |
|---|---|---|---|---|---|---|
| Be | DMQMC | $5 \times 10^5$ | $5 \times 10^5$ | $1.6174(3) \times 10^5$ | $5.04704(8) \times 10^5$ | 100 |
| Be | IP-DMQMC | $5 \times 10^5$ | $5.63(2) \times 10^5$ | $5.204(5) \times 10^5$ | $6.03(1) \times 10^5$ | 100 |
| Be | PIP-DMQMC | $5 \times 10^5$ | $6.9575(2) \times 10^5$ | $5.27(1) \times 10^5$ | $7.0385(2) \times 10^5$ | 100 |
| $BeH_2$ | DMQMC | $1 \times 10^7$ | $1 \times 10^7$ | $4.4008(2) \times 10^6$ | $1.010706(7) \times 10^7$ | 100 |
| $BeH_2$ | IP-DMQMC | $1 \times 10^7$ | $1.067(2) \times 10^7$ | $1.067(2) \times 10^7$ | $1.416(3) \times 10^7$ | 100 |
| $BeH_2$ ($\beta_T = 1.0$) | PIP-DMQMC | $1 \times 10^7$ | $1.29427(1) \times 10^7$ | $1.29427(1) \times 10^7$ | $1.696(1) \times 10^7$ | 100 |
| $BeH_2$ ($\beta_T = 2.0$) | PIP-DMQMC | $1 \times 10^7$ | $1.190442(9) \times 10^7$ | $1.190442(9) \times 10^7$ | $1.51(2) \times 10^7$ | 100 |
| $BeH_2$ ($\beta_T = 5.0$) | PIP-DMQMC | $1 \times 10^7$ | $1.055211(5) \times 10^7$ | $1.055211(5) \times 10^7$ | $1.396654(8) \times 10^7$ | 100 |
| $BeH_2$ ($\beta_T = 10.0$) | PIP-DMQMC | $1 \times 10^7$ | $1.004129(1) \times 10^7$ | $1.004129(1) \times 10^7$ | $1.365538(3) \times 10^7$ | 100 |
| $BeH_2$ ($\beta_T = 20.0$) | PIP-DMQMC | $1 \times 10^7$ | $1.0000840(3) \times 10^7$ | $1.0000840(3) \times 10^7$ | $1.363041(3) \times 10^7$ | 100 |
| CO | DMQMC | $5 \times 10^5$ | $5 \times 10^5$ | $4.2509(3) \times 10^5$ | $5.1481(1) \times 10^5$ | 100 |
| CO | IP-DMQMC | $5 \times 10^5$ | $5.146(7) \times 10^5$ | $5.145(7) \times 10^5$ | $7.083(6) \times 10^5$ | 100 |
| CO | PIP-DMQMC | $5 \times 10^5$ | $5.9656(2) \times 10^5$ | $5.9656(2) \times 10^5$ | $7.7081(3) \times 10^5$ | 100 |
| equilibrium $H_4$ | DMQMC | $1 \times 10^7$ | $1 \times 10^7$ | $7.5389(2) \times 10^6$ | $1.017650(6) \times 10^7$ | 100 |
| equilibrium $H_4$ | IP-DMQMC | $1 \times 10^7$ | $1.057(3) \times 10^7$ | $1.057(3) \times 10^7$ | $1.556(3) \times 10^7$ | 100 |
| equilibrium $H_4$ | PIP-DMQMC | $1 \times 10^7$ | $1.27493(1) \times 10^7$ | $1.27493(1) \times 10^7$ | $1.7780(3) \times 10^7$ | 100 |
| equilibrium $H_8$ | DMQMC | $1 \times 10^7$ | $1 \times 10^7$ | $7.9200(1) \times 10^6$ | $1.18805(1) \times 10^7$ | 100 |
| equilibrium $H_8$ | IP-DMQMC | $1 \times 10^7$ | $1.055(2) \times 10^7$ | $1.055(2) \times 10^7$ | $1.529(4) \times 10^7$ | 100 |
| equilibrium $H_8$ | PIP-DMQMC | $1 \times 10^7$ | $1.265385(9) \times 10^7$ | $1.17411(1) \times 10^7$ | $1.92093(1) \times 10^7$ | 100 |
| stretched $H_8$ | DMQMC | $1 \times 10^7$ | $1 \times 10^7$ | $9.20033(9) \times 10^6$ | $1.37374(1) \times 10^7$ | 100 |
| stretched $H_8$ | IP-DMQMC | $1 \times 10^7$ | $1.072(2) \times 10^7$ | $1.072(2) \times 10^7$ | $1.627(4) \times 10^7$ | 100 |
| stretched $H_8$ | PIP-DMQMC | $1 \times 10^7$ | $1.29609(1) \times 10^7$ | $1.29609(1) \times 10^7$ | $1.95221(1) \times 10^7$ | 100 |
| HCN | DMQMC | $1 \times 10^7$ | $1 \times 10^7$ | $8.5086(2) \times 10^6$ | $1.07210(1) \times 10^7$ | 100 |
| HCN | IP-DMQMC | $1 \times 10^7$ | $1.027(1) \times 10^7$ | $1.027(1) \times 10^7$ | $1.544(2) \times 10^7$ | 100 |
| HCN | PIP-DMQMC | $1 \times 10^7$ | $1.148177(8) \times 10^7$ | $1.148177(8) \times 10^7$ | $1.72265(2) \times 10^7$ | 100 |
| LiF | DMQMC | $5 \times 10^6$ | $5 \times 10^6$ | $2.2359(1) \times 10^6$ | $5.06943(6) \times 10^6$ | 100 |
| LiF | IP-DMQMC | $5 \times 10^6$ | $5.96(4) \times 10^6$ | $5.47(2) \times 10^6$ | $7.26(3) \times 10^6$ | 100 |
| LiF | PIP-DMQMC | $5 \times 10^6$ | $1.01199(3) \times 10^7$ | $6.819(1) \times 10^6$ | $1.05079(3) \times 10^7$ | 100 |
| $N_2$ | DMQMC | $5 \times 10^5$ | $5 \times 10^5$ | $2.0931(3) \times 10^5$ | $5.16368(6) \times 10^5$ | 100 |
| $N_2$ | IP-DMQMC | $5 \times 10^5$ | $5.102(6) \times 10^5$ | $5.100(5) \times 10^5$ | $6.752(4) \times 10^5$ | 100 |
| $N_2$ | PIP-DMQMC | $5 \times 10^5$ | $5.7298(1) \times 10^5$ | $5.226(5) \times 10^5$ | $7.011(2) \times 10^5$ | 100 |
| $HBCH_2$ | i-PIP-DMQMC | $5 \times 10^4$ | $5.63503(7) \times 10^4$ | $5.63503(7) \times 10^4$ | $1.21416(5) \times 10^5$ | 5000 |
| $HBCH_2$ | i-PIP-DMQMC | $5 \times 10^5$ | $5.62867(7) \times 10^5$ | $5.62867(7) \times 10^5$ | $1.19044(4) \times 10^6$ | 500 |
| $HBCH_2$ | i-PIP-DMQMC | $5 \times 10^6$ | $5.62789(8) \times 10^6$ | $5.62789(8) \times 10^6$ | $1.11797(4) \times 10^7$ | 50 |
| $HBCH_2$ | i-PIP-DMQMC | $5 \times 10^7$ | $5.62788(6) \times 10^7$ | $5.4373(3) \times 10^7$ | $1.041386(8) \times 10^8$ | 4 |
| $H_2O$ | i-PIP-DMQMC | $5 \times 10^6$ | $5.9527(1) \times 10^6$ | $5.9527(1) \times 10^6$ | $3.1131(1) \times 10^7$ | 50 |
| $H_2O$ | i-PIP-DMQMC | $1 \times 10^7$ | $1.19051(2) \times 10^7$ | $1.19051(2) \times 10^7$ | $6.1354(2) \times 10^7$ | 25 |
| $H_2O$ | i-PIP-DMQMC | $2 \times 10^7$ | $2.38102(5) \times 10^7$ | $2.38102(5) \times 10^7$ | $1.20465(4) \times 10^8$ | 10 |
| $H_2O$ | i-PIP-DMQMC | $5 \times 10^7$ | $5.95245(7) \times 10^7$ | $5.95245(7) \times 10^7$ | $2.9222(1) \times 10^8$ | 5 |
| $H_2O$ | i-PIP-DMQMC | $5 \times 10^8$ | $5.95256(2) \times 10^8$ | $5.95256(2) \times 10^8$ | $2.66165(2) \times 10^9$ | 4 |
| $CH_4$ | i-PIP-DMQMC | $5 \times 10^6$ | $5.57370(5) \times 10^6$ | $5.57370(5) \times 10^6$ | $3.5362(1) \times 10^7$ | 50 |
| $CH_4$ | i-PIP-DMQMC | $1 \times 10^7$ | $1.11475(1) \times 10^7$ | $1.11475(1) \times 10^7$ | $7.0704(3) \times 10^7$ | 25 |
| $CH_4$ | i-PIP-DMQMC | $2 \times 10^7$ | $2.22946(3) \times 10^7$ | $2.22946(3) \times 10^7$ | $1.41340(5) \times 10^8$ | 10 |
| $CH_4$ | i-PIP-DMQMC | $5 \times 10^7$ | $5.57365(1) \times 10^7$ | $5.57365(1) \times 10^7$ | $3.5287(1) \times 10^8$ | 5 |
| $CH_4$ | i-PIP-DMQMC | $5 \times 10^8$ | $5.57373(2) \times 10^8$ | $5.57373(2) \times 10^8$ | $3.48413(2) \times 10^9$ | 5 |

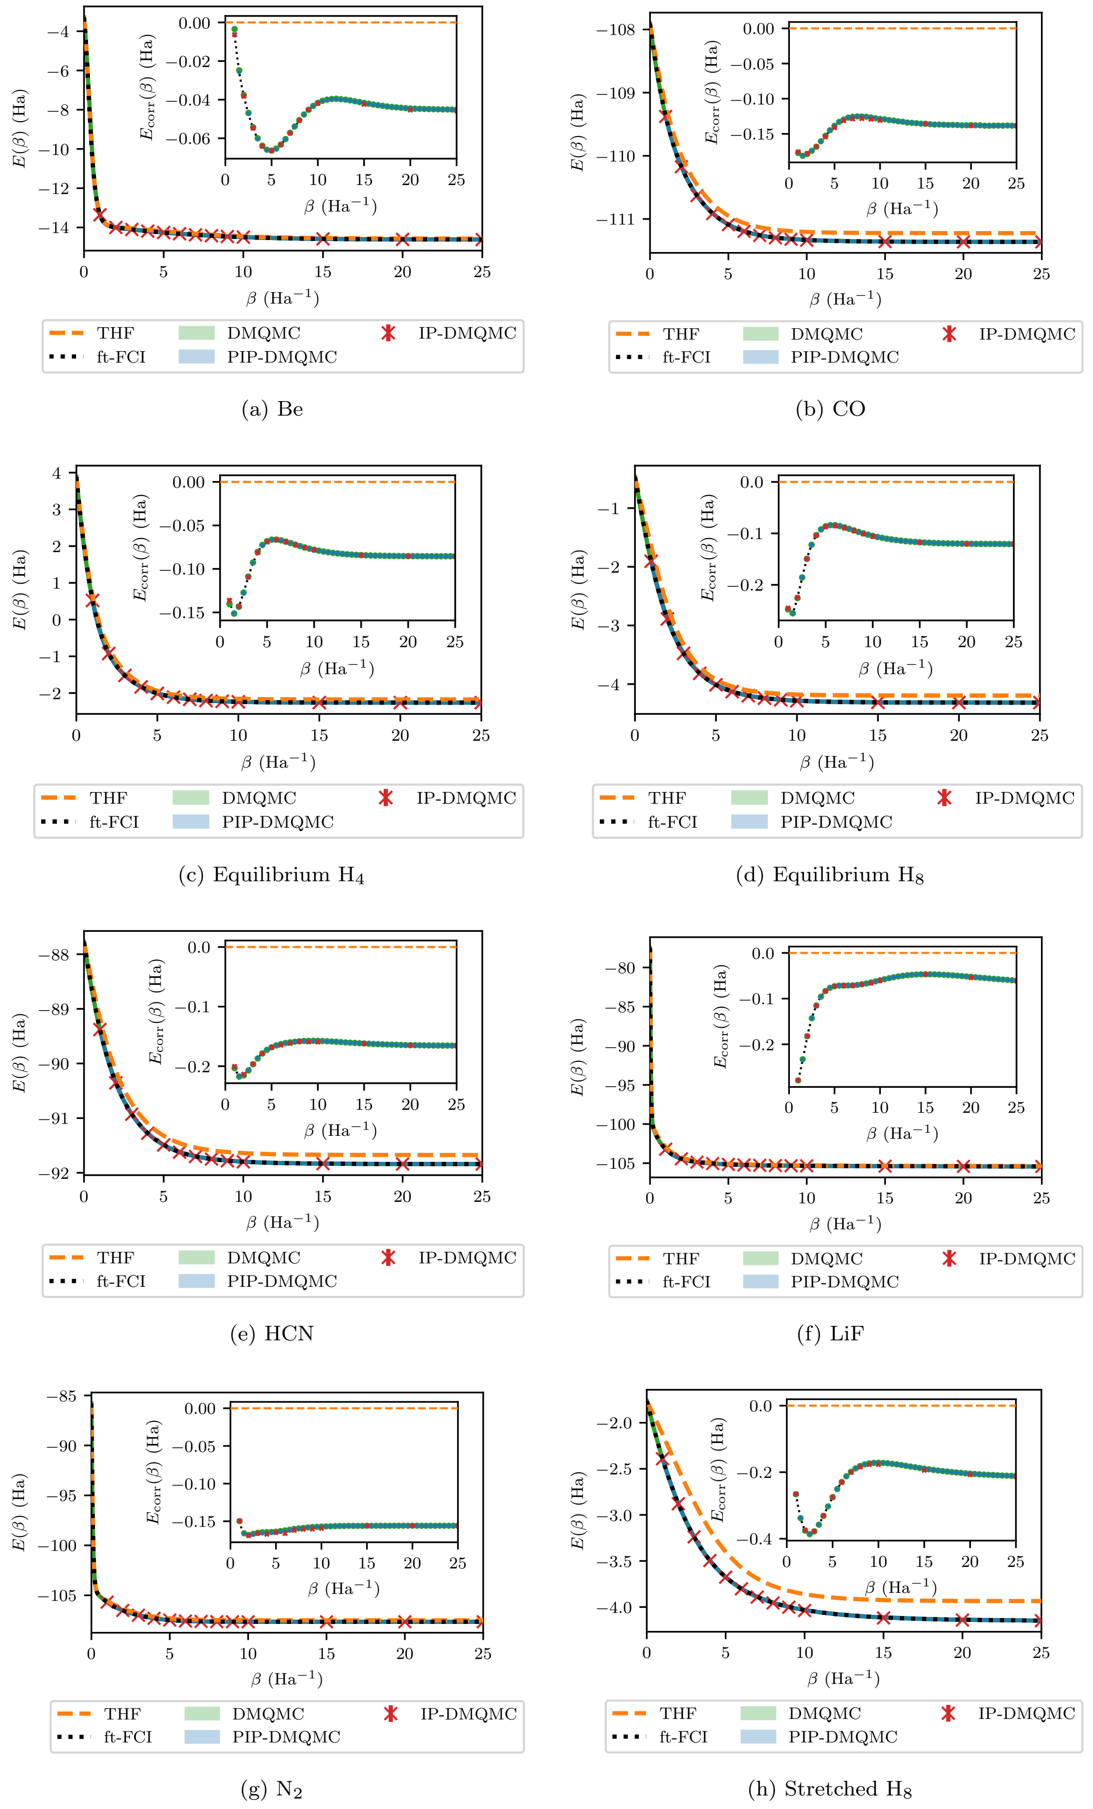


Figure 1. Energies from asymmetric PIP-DMQMC (blue), DMQMC (green), IP-DMQMC (red), ft-FCI (black dashed) and THF (orange dashed) are shown. The correlation energy calculated with the various methods difference to THF are shown in the inset. The PIP-DMQMC simulations were initialized with $\beta_T = 1.0$, allowing data collection at $\beta \geq 1.0$.

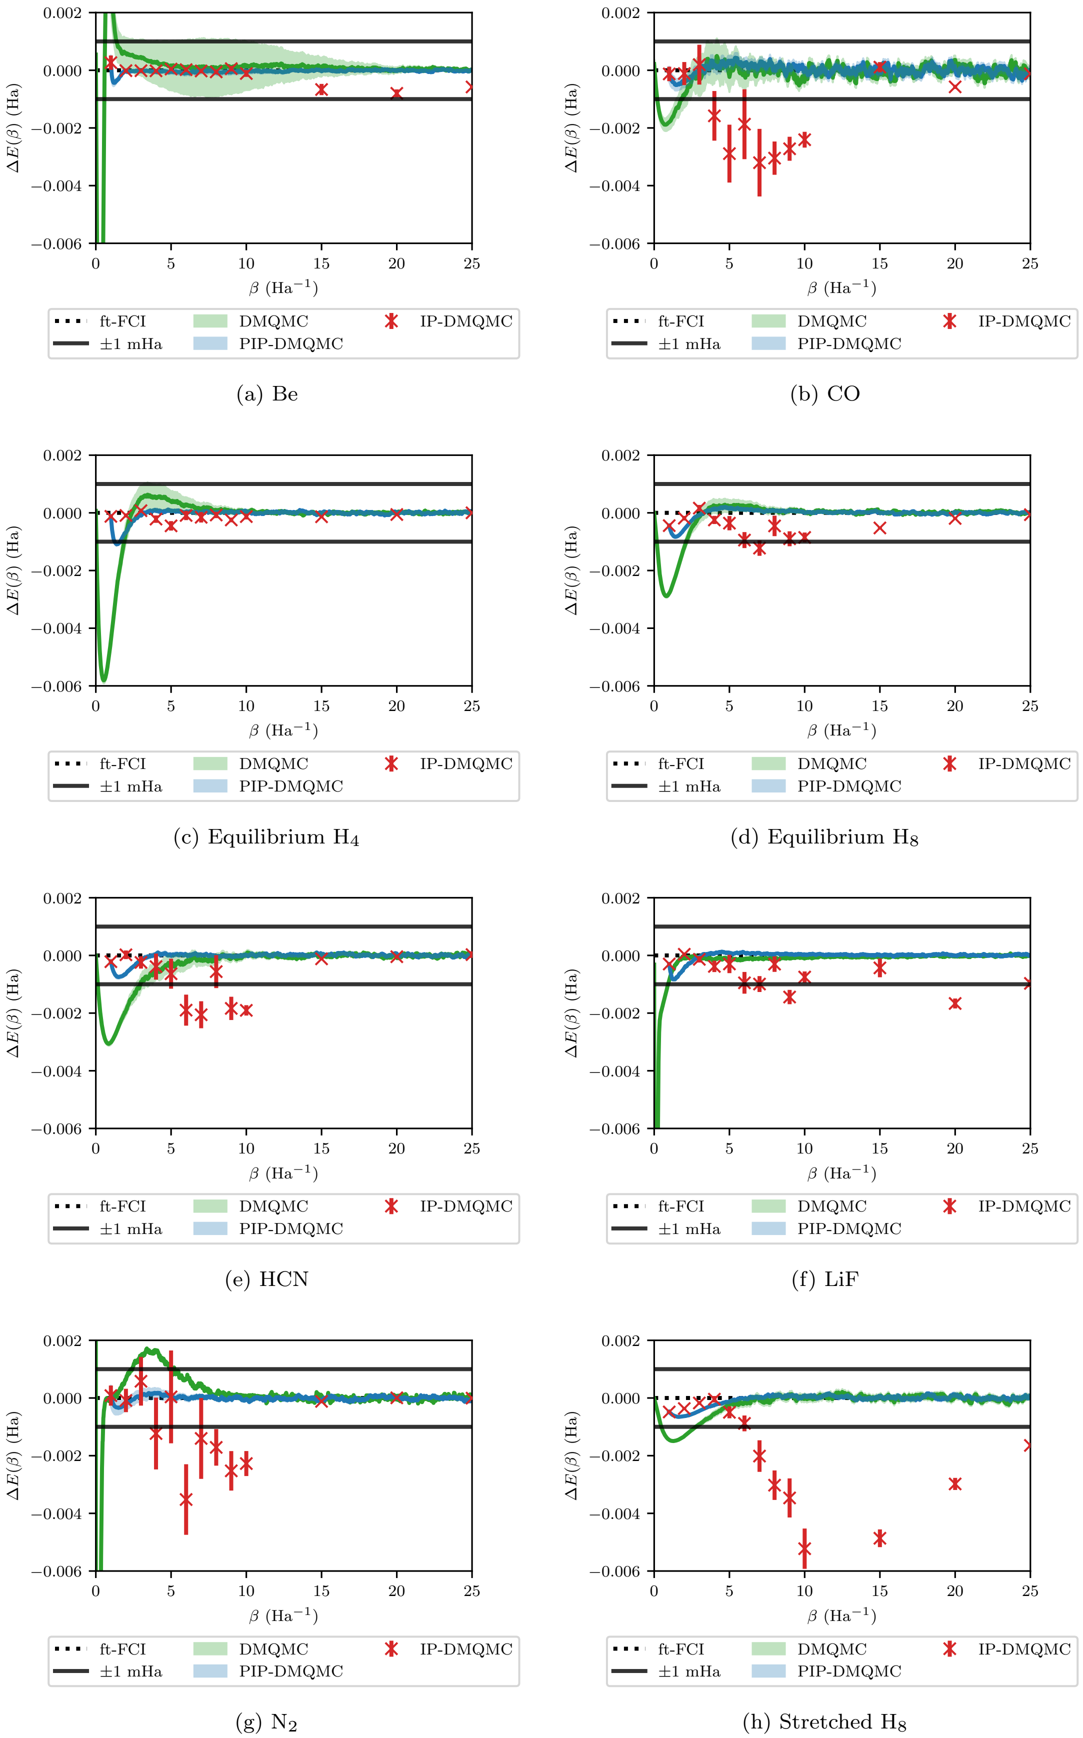


Figure 2. Difference to the exact result (ft-FCI) for PIP-DMQMC (blue), DMQMC (green), IP-DMQMC (red). Solid black lines shown to indicate ±1 mHa. The PIP-DMQMC simulations were initialized with $\beta_T = 1.0$, allowing data collection at $\beta \geq 1.0$.

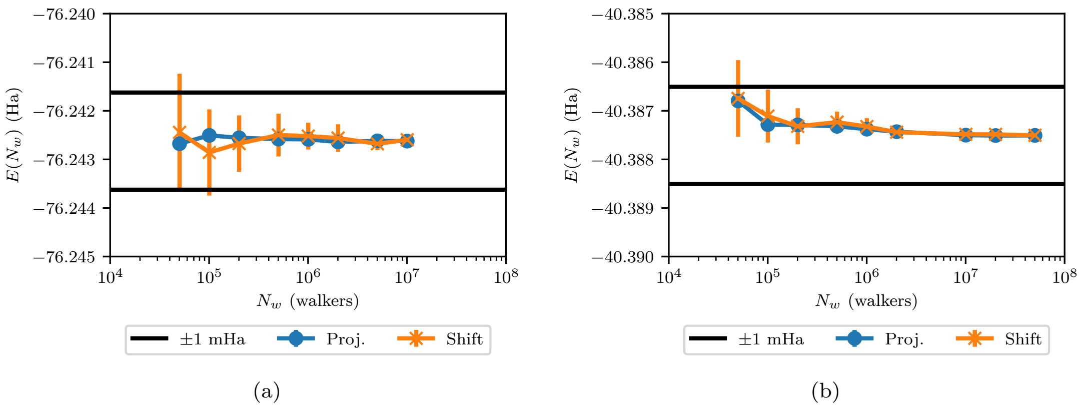


Figure 3. Energies from initiator FCIQMC for increasing walker populations for (a) $H_2O$/cc-pVDZ and (b) $CH_4$/cc-pVDZ. The shift and projected estimates of the energy agree within a $\sigma$ of error for $N_w = 1 \times 10^7$ in the water system and $N_w = 5 \times 10^7$ in the methane system. The black lines (±1 mHa) are plotted relative to the largest walker populations projected energy.
